# Supplementary material for: Unified Gas-Kinetic Particle Method for Frequency-dependent Radiation Transport
Source: arXiv:2301.06110 source file (2023-01-15)
Supplement: Supplementary file 1 [file article_appendix.tex]

% vim: tw=70:spell
\appendix

\section{Appendix}

\subsection{Boundary flux}
